# Supplementary material for: Computing Covers under Substring Consistent Equivalence Relations
Source: arXiv:2002.06764 source file (2020-07-30)
Supplement: Supplementary file 1 [file appendix.tex]

\section{Proofs of lemmas}\label{apdx:proofs}

%%%%%%%%%%
% Preliminaries
%%%%%%%%%%

\barrayproperty*
\PROOFbarrayproperty{}
%%%%%%%%%%
% Cover
%%%%%%%%%%
%\setcounter{lemma}{\ref{lem:coverisbordercover}}
%\addtocounter{lemma}{-1}
\coverisbordercover*
%\begin{lemma}%\label{lem:coverisbordercover}
%	For any $C \in \Cov(T)$ of length $m$ and $B \in \Bord(T)$ of length $b$ such that $m \le b$,
%	$C \in \Cov(B)$.
%\end{lemma}
\PROOFcoverisbordercover{}

\shortcoverlong*
%\begin{lemma}%\label{lem:shortcoverlong}
%    For any $C,C'\in \Cov(T)$ such that $|C| \le |C'|$,
%	$C \in \Cov(C')$.
%\end{lemma}
\PROOFshortcoverlong{}

\covercover*
%\begin{lemma}%\label{lem:covercover}
%	If $C \in \Cov(T)$ and
%	$C' \in \Cov(C)$, 
%	then $C' \in \Cov(T)$.
%\end{lemma}
\PROOFcovercover{}

\forreach*
%\begin{lemma}%\label{lem:forreach}
%	For any strings $T$ of length $n$ and $C$ of length $m$,
%	$C$ is a proper \ACover{} of $T$ iff $C \in \Bord(T)$ and $C \in \Cov(T[:n-i])$ for some $1 \le i \le m$.
%\end{lemma}
\PROOFforreach{}

%%%%%%%%%%
% LCover
%%%%%%%%%%

\clearlylseed*
%\begin{lemma}%\label{lem:clearlylseed}
%	For any $1 \le i \le n$ and $i-\Border_T[i] \le j \le i$,
%    we have $T[:j] \in \LSeed(T[:i])$.
%\end{lemma}
%\PROOFclearlyseed{}

\deadproperty*
%\PROOFdeadproperty{}

\section{Comparing Li \& Smyth's algorithm and ours}\label{apdx:comparison}
Algorithm~\ref{alg:LiSmyth} shows Li \& Smyth's algorithm for computing longest cover arrays.
Slight differences from Algorithm~\ref{alg:lcover_increasing} are in \Cref{algln:decreasing} of the main algorithm and in \Cref{alg:dead_check} of $\SetDead$.
\begin{algorithm2e}[t]
	\caption{Li and Smyth's original algorithm}
	\label{alg:LiSmyth}
	\SetVlineSkip{0.5mm}
	let $T$ be the input text of length $n$\;
	let $\Border$ be the border array of $T$\;
    $\LCover[0] \leftarrow -1$\;
	$\Dead[i] \leftarrow \False$,
	$\LiveChildren[i] \leftarrow 0$,
	$\LargestLive[i] \leftarrow i$ for $0 \le i \le n$\;
	\For{$1 \le i \le n$}{
		\If{$\Dead[\Border[i]] = \True$}{
			$\LargestLive[\Border[i]] \leftarrow \LargestLive[\LCover[\Border[i]]]$\;
		}
		$\LCover[i] \leftarrow \LargestLive[\Border[i]]$\;
		$\LiveChildren[\LCover[i]] \leftarrow \LiveChildren[\LCover[i]] + 1$\;\label{algln:cp1}
		\If{$i > 1$}{
			$c_1 \leftarrow i-\Border[i]$\;
			$c_2 \leftarrow (i-1) - \Border[i-1]$\;
            \For{$j$ \textbf{\textup{from}} $c_1-1$ \textbf{\textup{downto}} $c_2$\label{algln:decreasing}}{
    			$\SetDead(j)$\;
            }
		}
	}
\end{algorithm2e}
\begin{algorithm2e}[t]
	\caption{$\SetDead(j)$ by Li and Smyth}
    \label{alg:LS_dead}
	\SetVlineSkip{0.5mm}
	\If{$\LiveChildren[j] = 0$ and $\Dead[j]=\False$}{\label{alg:dead_check}
		$\Dead[j] \leftarrow \True$\;
		$\LiveChildren[\LCover[j]] \leftarrow \LiveChildren[\LCover[j]] - 1$\;
		$\SetDead(\LCover[j])$\;
	}
\end{algorithm2e}

Let us observe the difference of the behaviors of those algorithm using a text $T=\mtt{aab}$.
Right after executing \Cref{algln:cp1} in the third iteration of the outer \textbf{for} loop ($i=3$), both algorithms have 
\[
\begin{array}{c|cccc}
	&	0	& 1 & 2 & 3
\\ \hline
\Border & 0 & 0 & 1 & 0
\\ \hline
\Dead		& \mbf{F} & \mbf{F} &\mbf{F} &\mbf{F}
\\
\LiveChildren & 2 & 1 & 0 & 0
\\
\LargestLive & 0 & 1  & 2 & 3
\\
\LCover & -1 & 0 & 1 & \bot
\end{array}
\]
where $\mtt{T}$, $\mtt{F}$ and $\bot$ denote $\True$, $\False$ and undefined, respectively.
Let $c_1 = 3-\Border[3] = 3$ and $c_2 = 2-\Border[2]=1$.
Both algorithms call $\SetDead(j)$ for $j \in \{1,2\}$ but in the reverse order. 

\Cref{alg:lcover_increasing} calls $\SetDead(1)$ first.
Since $\LiveChildren[1] = 1$, $\SetDead(1)$ does nothing.
Next, \Cref{alg:lcover_increasing} calls $\SetDead(2)$, where $\LiveChildren[2] = 0$.
Then $\Dead[2]$ is set to $\True$ and $\LiveChildren[\LCover[2]]=\LiveChildren[1]$ is decremented to $0$.
Subsequently $\SetDead(\LCover[2]) = \SetDead(1)$ is called recursively.
Now $\LiveChildren[1] = 0$, so the algorithm proceeds.
$\Dead[1]$ becomes $\True$ and $\LiveChildren[\LCover[1]]=\LiveChildren[0]$ will be decremented to $1$.
Then $\SetDead(0)$ is called but by $\LiveChildren[0]=1$, the recursion stops.
The calculation process of those arrays are summarized as follows.
\[
\begin{array}{c|cccc}
	&	0	& 1 & 2 & 3
\\ \hline
\Border & 0 & 0 & 1 & 0
\\ \hline
\Dead		& \mtt{F} & \mtt{F} &\mbf{T} &\mtt{F}
\\
\LiveChildren & 2 & \mbf{0} & 0 & 0
\\
\LargestLive & 0 & 1  & 2 & 3
\\
\LCover & -1 & 0 & 1 & \bot
\end{array}
\quad \longrightarrow \quad
\begin{array}{c|cccc}
	&	0	& 1 & 2 & 3
\\ \hline
\Border & 0 & 0 & 1 & 0
\\ \hline
\Dead		& \mtt{F} & \mbf{T} &\mtt{T} &\mtt{F}
\\
\LiveChildren & \mbf{1} & 0 & 0 & 0
\\
\LargestLive & 0 & 1  & 2 & 3
\\
\LCover & -1 & 0 & 1 & \bot
\end{array}
\]

On the other hand, \Cref{alg:LiSmyth} calls $\SetDead(2)$ first.
Since $\LiveChildren[2] = 0$ and $\Dead[2]=\False$,
 the algorithm sets $\Dead[2]$ to $\True$ and decrements $\LiveChildren[\LCover[2]]=\LiveChildren[1]$ to $0$.
Subsequently $\SetDead(\LCover[2]) = \SetDead(1)$ is called recursively.
Since $\LiveChildren[1] = 0$ and $\Dead[1]=\False$, 
 the algorithm sets $\Dead[1]$ to $\True$ and decrements $\LiveChildren[\LCover[1]]=\LiveChildren[0]$ to $1$.
 Subsequently $\SetDead(0)$ is called but by $\LiveChildren[0]=1$, the recursion stops.
Next, \Cref{alg:LiSmyth} calls $\SetDead(1)$.
Since $\LiveChildren[1]=0$ but $\Dead[1]=\True$, $\SetDead(1)$ does nothing.

As a consequence, both algorithms get the same arrays.
However, we observe that checking $\Dead$ value is necessary for Li \& Smyth's $\SetDead$ (\Cref{alg:LS_dead}).
If this condition was lifted, when \Cref{alg:LiSmyth} calls $\SetDead(1)$, 
the algorithm decrements $\LiveChildren[\LCover[1]] = \LiveChildren[0]$ to $0$,
where we have no right invariants any more.
Moreover, it will call $\SetDead(0)$ and try to access $\LiveChildren[\LCover[0]]=\LiveChildren[-1]$.
\[
\begin{array}{c|cccc}
	&	0	& 1 & 2 & 3
\\ \hline
\Border & 0 & 0 & 1 & 0
\\ \hline
\Dead		& \mbf{T} & \mtt{T} &\mtt{T} &\mtt{F}
\\
\LiveChildren & \mbf{0} & 0 & 0 & 0
\\
\LargestLive & 0 & 1  & 2 & 3
\\
\LCover & -1 & 0 & 1 & \bot
\end{array}
\]
On the other hand, our modification algorithm does not need to check $\Dead[j]$ when $\SetDead(j)$ is called,
since $\Dead[j]=\False$ is always guaranteed, as we have shown in the proof of Theorem~\ref{thm:lcover}.

We argued that we can remove the array $\Dead$ from our algorithm.
On the other hand, one cannot remove $\Dead$ from Li \& Smyth's as we have observed above.
The tidy invariant on $\Dead$ that holds at the end of the $i$-th iteration of the outer \textbf{for} loop of the main algorithm does not hold during executions of $\SetDead$, particularly when their algorithm checks the value of $\Dead[j]$.

%
%\section{A minor error in Li \& Smyth's paper}\label{apdx:LS_error}
%Li and Smyth claimed that $\LargestLive[j] = \LLive_T(j,i)$ holds not only for $j \le \Border_T[i]$, but for all $j \le i$ in~\cite{Li2002}.
%We give a counterexample to this claim.
%Consider $T = \mathtt{abaabc}$ on $\Sigma = \{{\tt a,b,c}\}$ under the identity relation.
%At the end of the sixth iteration of their algorithm,
%$\LargestLive = [0,0,3,4,5,0]$ and $\Dead = [{\tt T,T,T,T,T,F}]$, where $\mtt{T} = \textbf{True}$ and $\mtt{F} = \textbf{False}$.
%If it did hold $\LargestLive[j] = \LLive_T(j,i)$ for $j \le i$, it must be $\LargestLive = [0,0,0,0,0,6]$.
%
